# Supplementary material for: Stochastic Thermodynamics of Brownian motion in Temperature Gradient
Source: arXiv:2308.15764 source file (2024-02-21)
Supplement: Supplementary file 1 [file supplementary-temperature-gradient.pdf]

# Supplementary Information: Stochastic Thermodynamics of Thermophoresis

Mingnan Ding<sup>1,\*</sup>, Jun Wu<sup>1</sup>, and Xiangjun Xing<sup>1,2,3†</sup>

<sup>1</sup>*Wilczek Quantum Center, School of Physics and Astronomy,  
Shanghai Jiao Tong University, Shanghai, 200240 China*

<sup>2</sup>*T.D. Lee Institute, Shanghai Jiao Tong University, Shanghai, 200240 China*

<sup>3</sup>*Shanghai Research Center for Quantum Sciences, Shanghai 201315, China*

(Dated: April 17, 2023)

## Abstract

We supply some details of analytic calculation and numerical simulation.

PACS numbers:

---

\*Electronic address: [dmnphy@sjtu.edu.cn](mailto:dmnphy@sjtu.edu.cn)

†Electronic address: [xxing@sjtu.edu.cn](mailto:xxing@sjtu.edu.cn)

## I. PROOF OF EQ. (5)

Here we explain how to take ensemble average of Eq. (4) to obtain Eq. (5). Here ensemble average means average both over noises and over pdf of  $\mathbf{x}$ . Firstly, we note that the Stratonovich product in Eq. (4) is defined as

$$\begin{aligned} -\partial_i U \circ dx^i &= -\partial_i U(\mathbf{x} + d\mathbf{x}/2) dx^i \\ &= -\partial_i U(\mathbf{x}) dx^i - \frac{1}{2} \partial_i \partial_j U(\mathbf{x}) dx^i dx^j, \end{aligned} \quad (1.1)$$

where in the second step we expanded up to the order  $dx^2$  because  $d\mathbf{x} \sim \sqrt{dt}$ , and that we only need to keep terms up to order  $dt$ . Now using the Langevin equation (1) in the preceding equation, and ignoring all terms in the form of  $dt^2, dt dW^i$ , as well as using the property of Wiener noise  $(dW^i)^2 = dt$ , finally averaging over noises and noticing  $\langle dW^i(t) \rangle = 0$ , we obtain:

$$\begin{aligned} \langle -\partial_i U \circ dx^i \rangle &= \frac{T}{\gamma} (\partial_i U)^2 dt - \left( \partial_i \frac{T}{\gamma} \right) \partial_i U dt - \frac{T}{\gamma} \partial_i^2 U dt \\ &= (\partial_i - (\partial_i U)) \frac{T}{\gamma} \partial_i U. \end{aligned} \quad (1.2)$$

Now we multiply the preceding equation by  $p(\mathbf{x}, t)$  and integrate over  $\mathbf{x}$ :

$$\langle\langle -\partial_i U \circ dx^i \rangle\rangle = \int_{\mathbf{x}} p(\mathbf{x}, t) (\partial_i - (\partial_i U)) \frac{T}{\gamma} \partial_i U. \quad (1.3)$$

Integrating by parts once, we obtain Eq. (5). In the l.h.s. of the preceding equation,  $\langle\langle \cdot \rangle\rangle$  means average both over noises and over pdf of  $\mathbf{x}$ .

## II. PROOF OF EQ. (11)

Consider the forward trajectory  $\mathbf{x}(t)$  with  $t \in [0, \tau]$ , we may approximate it using the discrete sequence  $\mathbf{x}_N \mathbf{x}_{N-1} \cdots \mathbf{x}_0$ , where  $\mathbf{x}_0 = \mathbf{x}(0), \mathbf{x}_N = \mathbf{x}(\tau)$ , and the time propagates from right to left. The backward trajectory  $\tilde{\mathbf{x}}(t)$  can be similarly broken into N segments. For each segment  $\mathbf{x}_{k+1} \mathbf{x}_k$  of the forward trajectory, we have a relation (c.f. Eq. (10) of the main text):

$$\begin{aligned} \log \frac{P_F(\mathbf{x}_{k+1} | \mathbf{x}_k; dt)}{P_B(\mathbf{x}_k | \mathbf{x}_{k+1}; dt)} &= U(\mathbf{x}_{k+1}, \lambda_k) - U(\mathbf{x}_k, \lambda_k) \\ &= \nabla U(\mathbf{x}_k, \lambda_k) \circ d\mathbf{x}_k \end{aligned} \quad (2.1)$$

Now consider the following products:

$$p_F[\gamma|\gamma_0] = p_F(\mathbf{x}_N|\mathbf{x}_{N-1}) \cdots p_F(\mathbf{x}_1|\mathbf{x}_0); \quad (2.2)$$

$$p_B[\tilde{\gamma}|\tilde{\gamma}_0] = p_F(\mathbf{x}_0|\mathbf{x}_1) \cdots p_F(\mathbf{x}_{N-1}|\mathbf{x}_N). \quad (2.3)$$

Whilst Eq. (??) can be understood as the discretized probability density of the forward trajectory  $\gamma = \mathbf{x}(t)$  conditioned on the initial state  $\gamma_0 = \mathbf{x}_0$ , Eq. (??) can be understood as the discretized probability density of the backward trajectory  $\tilde{\gamma} = \mathbf{x}(\tau - t)$  conditioned on the initial state  $\tilde{\gamma}_0 = \mathbf{x}_N$ . Now taking the ratio between Eqs. (??) and (??), and using Eq. (??) for each step, we obtain

$$\log \frac{P_F[\gamma|\gamma_0]}{P_B[\tilde{\gamma}|\tilde{\gamma}_0]} = - \int \partial_i U(\mathbf{x}, \lambda) \circ dx^i = - \int_{\gamma} d_{\mathbf{x}} U. \quad (2.4)$$

Now recall that in the main text we choose the initial distribution of the forward process as the steady-state distribution Eq. (9a), and the initial distribution of the backward process as the steady-state distribution Eq. (9b), which we rewrite below

$$p_F(\gamma_0) = e^{-U(\mathbf{x}_0, \lambda_i)}, \quad (2.5a)$$

$$p_B(\tilde{\gamma}_0) = e^{-U(\mathbf{x}_N, \lambda_f)}, \quad (2.5b)$$

Combining Eqs. (??) with (??) we obtain the following relation between the unconditional path probability of the forward process and that of the backward process:

$$\log \frac{P_F[\gamma]}{P_B[\tilde{\gamma}]} = \log \frac{P_F[\gamma|\gamma_0]p_F(\gamma_0)}{P_B[\tilde{\gamma}|\tilde{\gamma}_0]p_B(\tilde{\gamma}_0)} \quad (2.6)$$

$$= U(\mathbf{x}_f, \lambda_f) - U(\mathbf{x}_i, \lambda_i) - \int_{\gamma} d_{\mathbf{x}} U. \quad (2.7)$$

This is the first equality of Eq. (11). But since the difference  $U(\mathbf{x}_f, \lambda_f) - U(\mathbf{x}_i, \lambda_i)$  can be written as the integral  $\int_{\gamma} (d_{\mathbf{x}} U + d_{\lambda} U)$ , we may also write the preceding equation as

$$\log \frac{P_F[\gamma]}{P_B[\tilde{\gamma}]} = \int_{\gamma} d_{\lambda} U, \quad (2.8)$$

which is the last equality of Eq. (11).

Recall that the differential excess entropy change of environment is defined as Eq. (4) in the main text. The excess entropy change of environment along the entire forward trajectory (in the forward process) is then given by

$$\Sigma_F^{\text{ex}}[\gamma] = - \int_{\gamma} d_{\mathbf{x}} U. \quad (2.9)$$

On the other hand, the change of *stochastic entropy* [?] of the system along the forward trajectory is defined as

$$\begin{aligned}\Delta\mathcal{S}^{\text{ST}} &= -\log p_{\text{F}}(\mathbf{x}_N) + \log p_{\text{F}}(\mathbf{x}_0) \\ &= -\log p_{\text{B}}(\mathbf{x}_N) + \log p_{\text{F}}(\mathbf{x}_0) \\ &= U(\mathbf{x}_f, \lambda_f) - U(\mathbf{x}_i, \lambda_i).\end{aligned}\tag{2.10}$$

It then follows that the r.h.s. of Eq. (??) is the sum of the excess entropy change of the environment and the change of stochastic entropy of the system along the forward trajectory of the forward process. This is what we mean by the excess EP along the forward trajectory in the forward process. As one can easily see, it is also negative the excess EP along the backward trajectory in the backward process.

### III. METHODS OF MD SIMULATION

MD simulation were carried out using the LAMMPS package [?].

The 12-6 Lennard-Jones (LJ) pair potential truncated at zero potential is used to model the interaction between particles. Throughout this work all lengths are in units of the Lennard-Jones diameter  $\sigma_0$ , all energies are in units of the well-depth  $\epsilon_0$ , and the unit of time is  $\tau = \sqrt{m_0\sigma_0^2/\epsilon_0}$ , where  $m_0$  is the mass of the fluid particles. Boltzmann's constant is set equal to unity.

Let  $r$  be the distance between two particles. The interaction potential between two fluid particles is

$$V_{ff}(r) = \begin{cases} 4 \left[ \left( \frac{1}{r} \right)^{12} - \left( \frac{1}{r} \right)^6 \right], & r < 1, \\ 0, & \text{otherwise.} \end{cases}\tag{3.1}$$

The interaction potential between the Brownian particle and a fluid particle is

$$V_{cf}(r) = \begin{cases} 4 \left[ \left( \frac{2}{r} \right)^{12} - \left( \frac{2}{r} \right)^6 \right], & r < 2, \\ 0, & \text{otherwise.} \end{cases}\tag{3.2}$$

This amounts to choosing the diameters of fluid particles and the Brownian particle to be  $\sigma_0$  and  $3\sigma_0$  respectively.
